# Supplementary material for: ANON: Asymmetric and Narrated Outward-expansion Network for Photo Composition Repair
Source: arXiv:2611.37640 source file (2026-11-27)
Supplement: Supplementary file 1 [file suppl_labels.tex]

\makeatletter
\newlabel{sec:app_data}{{A}{1}{\texorpdfstring {\hskip -1em.~}{}Dataset construction details}{appendix.A}{}}
\newlabel{sec:app_data@cref}{{[appendix][1][2147483647]A}{[1][1][]1}}
\newlabel{sec:splits}{{A}{1}{Labels and splits}{section*.3}{}}
\newlabel{sec:splits@cref}{{[appendix][1][2147483647]A}{[1][1][]1}}
\newlabel{sec:app_rationale}{{B}{1}{\texorpdfstring {\hskip -1em.~}{}Rationale pipeline}{appendix.B}{}}
\newlabel{sec:app_rationale@cref}{{[appendix][2][2147483647]B}{[1][1][]1}}
\newlabel{tab:errtax}{{1}{1}{\textbf {Teacher errors by type.} The 1,658 remarks the judge made on the 1,552 reviewed rows, grouped by keyword, with the human verdict on each remark. Edge contact dominates, mostly a complete object close to a border written as cut; facing is the type where the judge itself is least reliable (18\% of its remarks not fully right)}{table.caption.8}{}}
\newlabel{tab:errtax@cref}{{[table][1][2147483647]1}{[1][1][]1}}
\newlabel{fig:errors}{{1}{2}{\textbf {How the teacher misdescribes a photo.} The two most common kinds of error in the training rationales, each shown with the teacher's observation (struck-out words were wrong, green words were added after the human verdict), the judge's remark and our decision. Top: a pictogram's facing direction is mirrored. Bottom: the prompt's word ``sits'' leaks into the description of a flying bird. Both were caught by the judge and corrected by hand; the trained planner inherits the same weak spots (\cref {sec:faithful})}{figure.caption.10}{}}
\newlabel{fig:errors@cref}{{[figure][1][2147483647]1}{[1][1][]2}}
\newlabel{tab:rejudge}{{2}{2}{\textbf {Blind re-judging of the corrected rows.} After the human-directed rewrite, the same judge re-read every corrected row without seeing the verdict. Almost every remaining remark re-asserts a reading the person had already overruled (left/right, bow/stern, back-to-camera), which is why the human makes the final decision}{table.caption.9}{}}
\newlabel{tab:rejudge@cref}{{[table][2][2147483647]2}{[1][1][]2}}
\newlabel{sec:app_training}{{C}{2}{\texorpdfstring {\hskip -1em.~}{}Training and inference details}{appendix.C}{}}
\newlabel{sec:app_training@cref}{{[appendix][3][2147483647]C}{[1][1][]2}}
\newlabel{sec:app_baselines}{{D}{2}{\texorpdfstring {\hskip -1em.~}{}Baseline reproduction}{appendix.D}{}}
\newlabel{sec:app_baselines@cref}{{[appendix][4][2147483647]D}{[1][2][]2}}
\newlabel{tab:regress}{{3}{3}{\textbf {Regression baselines.} A four-layer CNN trained from scratch and a two-layer MLP on the frozen global image embedding of CLIP ViT-B/16 or DINOv2 ViT-B/14, all trained on the same 15,000 crops (three seeds each), alongside the reference methods from \cref {tab:main}. They return the four numbers only}{table.caption.14}{}}
\newlabel{tab:regress@cref}{{[table][3][2147483647]3}{[1][3][]3}}
\newlabel{sec:app_realworld}{{E}{3}{\texorpdfstring {\hskip -1em.~}{}Hand-cropped frames and user study}{appendix.E}{}}
\newlabel{sec:app_realworld@cref}{{[appendix][5][2147483647]E}{[1][3][]3}}
\newlabel{tab:realworld81}{{4}{4}{\textbf {Hand-cropped real images.} Canvas IoU on the 81 hand-made crops (\cref {sec:app_realworld}), \anon {} against the strongest commercial baseline, both run once on the same crops. $\Delta $ is the paired difference with a 95\% bootstrap interval that resamples source photos, since crops of one photo are not independent. \anon {} is better on 60 of 81 crops and, taking each source photo's mean difference as one vote, on 33 of 48 photos (exact binomial test $p=0.013$)}{table.caption.18}{}}
\newlabel{tab:realworld81@cref}{{[table][4][2147483647]4}{[1][3][]4}}
\newlabel{sec:app_apps}{{F}{4}{\texorpdfstring {\hskip -1em.~}{}Additional applications}{appendix.F}{}}
\newlabel{sec:app_apps@cref}{{[appendix][6][2147483647]F}{[1][4][]4}}
\newlabel{sec:app_results}{{G}{4}{\texorpdfstring {\hskip -1em.~}{}Additional results}{appendix.G}{}}
\newlabel{sec:app_results@cref}{{[appendix][7][2147483647]G}{[1][4][]4}}
\newlabel{sec:app_stats}{{G.1}{4}{\texorpdfstring {\hskip -1em.~}{}Statistics and parse failures}{subsection.G.1}{}}
\newlabel{sec:app_stats@cref}{{[subappendix][1][2147483647,7]G.1}{[1][4][]4}}
\newlabel{sec:app_main}{{G.2}{5}{\texorpdfstring {\hskip -1em.~}{}Main results (\texorpdfstring {Sec.~\ref {sec:results}}{Sec. 4.2})}{subsection.G.2}{}}
\newlabel{sec:app_main@cref}{{[subappendix][2][2147483647,7]G.2}{[1][5][]5}}
\newlabel{sec:app_ablation}{{G.3}{5}{\texorpdfstring {\hskip -1em.~}{}Ablations (\texorpdfstring {Sec.~\ref {sec:ablation}}{Sec. 4.3})}{subsection.G.3}{}}
\newlabel{sec:app_ablation@cref}{{[subappendix][3][2147483647,7]G.3}{[1][5][]5}}
\newlabel{sec:app_faithful}{{G.4}{5}{\texorpdfstring {\hskip -1em.~}{}Rationale consistency and correctness (\texorpdfstring {Sec.~\ref {sec:faithful}}{Sec. 4.4})}{subsection.G.4}{}}
\newlabel{sec:app_faithful@cref}{{[subappendix][4][2147483647,7]G.4}{[1][5][]5}}
\newlabel{tab:breakdown}{{5}{6}{\textbf {Canvas mIoU per source and per tier.} The 300 test crops split by source photo set (96 / 100 / 104) and by crop tier (easy: subject pushed to the border; medium: cut; hard: a piece missing). All methods use the same configurations as in \cref {tab:main}. The hard tier is the lowest for every method except Qwen3.5-4B without ICL; no source is uniformly the hardest: \anon {} drops on PICD, most zero-shot VLMs on GAICD}{table.caption.23}{}}
\newlabel{tab:breakdown@cref}{{[table][5][2147483647]5}{[1][5][]6}}
\newlabel{tab:strata}{{6}{6}{\textbf {Canvas mIoU by how much the crop really needs.} The 300 test crops split by the mean true expansion over the four sides (no test crop needs more than 30\%). Bias is the mean predicted minus true side in percentage points. No large systematic expansion bias is observed for \anon {} within these synthetic strata, which contain no crop needing more than 30\%; Claude Opus 5.5 (w/ ICL) is ahead only on the crops that need the least}{table.caption.25}{}}
\newlabel{tab:strata@cref}{{[table][6][2147483647]6}{[1][5][]6}}
\newlabel{tab:addedarea}{{7}{6}{\textbf {IoU of the added region only.} Canvas IoU shares the input area between prediction and target, so a no-op already scores 0.593; here the input is removed from both canvases and the IoU is taken over the ring that is added. The ranking is unchanged and the gaps widen; $\Delta $ is the paired difference to \anon {} with a 95\% bootstrap interval over the 300 test crops}{table.caption.27}{}}
\newlabel{tab:addedarea@cref}{{[table][7][2147483647]7}{[1][5][]6}}
\newlabel{tab:textonly}{{8}{6}{\textbf {In-context examples with or without the example images.} Same 300 crops and protocol as \cref {tab:main}; in the text-only variant the nine examples are given as their answers alone and the model reads only the query image. Canvas mIoU moves by less than 0.01 either way; direction F1 is lower without the images for all three models, so the pictures carry some of the direction signal but little of the amount. The last three rows vary the protocol for the strongest model: two further example sets drawn with the same rule and other seeds (0.747 and 0.747 against 0.748), and a prompt that asks for two to four sentences of reasoning before the JSON (0.751, $+0.002$ with a 95\% interval of $-0.004$ to $+0.008$ against the plain (w/ ICL) run, not significant). Every variant stays below \anon {} (\res {ours_final@test300_seed0}{miou})}{table.caption.29}{}}
\newlabel{tab:textonly@cref}{{[table][8][2147483647]8}{[1][5][]6}}
\newlabel{tab:abl_mix}{{9}{7}{\textbf {Mixing rationale and numbers-only samples.} Final data (15,000 crops, final screened rationales) and the same 9,375 steps for every row, so the rows are comparable with \cref {tab:main}. Rows 1--3 give each crop 0, 1 or 2 numbers-only samples next to its rationale sample (row 2 is our final model); row 4 keeps the rationales of only 4,780 crops, with numbers-only samples for all 15,000; the last row has no rationales. All confidence intervals overlap}{table.caption.32}{}}
\newlabel{tab:abl_mix@cref}{{[table][9][2147483647]9}{[1][5][]7}}
\newlabel{tab:abl_geometry_direct}{{10}{7}{\textbf {The rewrites of \cref {tab:abl_geometry} applied to \anonnum {}.} Same definitions; the drops mirror those of \anon {}. The last two rows report separately retrained models: the same 15,000 crops and schedule with the label tied to one ratio for all four sides, or to one ratio per axis (left $=$ right, top $=$ bottom). Bold = best, underline = second}{table.caption.34}{}}
\newlabel{tab:abl_geometry_direct@cref}{{[table][10][2147483647]10}{[1][5][]7}}
\newlabel{sec:app_outpainter}{{G.5}{7}{\texorpdfstring {\hskip -1em.~}{}Outpainters (\texorpdfstring {Sec.~\ref {sec:generation}}{Sec. 4.5})}{subsection.G.5}{}}
\newlabel{sec:app_outpainter@cref}{{[subappendix][5][2147483647,7]G.5}{[1][7][]7}}
\newlabel{sec:app_metricval}{{G.6}{7}{\texorpdfstring {\hskip -1em.~}{}Validating automatic composition and aesthetic scorers}{subsection.G.6}{}}
\newlabel{sec:app_metricval@cref}{{[subappendix][6][2147483647,7]G.6}{[1][7][]7}}
\newlabel{tab:abl_geometry_opus}{{11}{8}{\textbf {Per-side decisions.} \anon {}: its predictions rewritten after the fact. Claude Opus 5.5 (w/ ICL): the same rewrite applied to its predictions, or the same rule stated in its prompt so it answers under the constraint. \emph {Dir.} = per-axis direction kept, \emph {Amount} = amount kept, \emph {Grid} = coarsening. Bold = best, underline = second, over all three groups}{table.caption.36}{}}
\newlabel{tab:abl_geometry_opus@cref}{{[table][11][2147483647]11}{[1][5][]8}}
\newlabel{tab:dirthr}{{12}{8}{\textbf {Direction F1 under a 5 / 10 / 15 / 20\% grow threshold.} Micro F1 over all $4N$ sides; the 10\% column is the one in \cref {tab:main}, with its precision and recall. The ordering of the trained models and the frontier VLMs holds from 10\% upward; at 5\%, where 63\% of the sides are positive, the numbers-only model and the constant prior move up because the task reduces to predicting ``grow''}{table.caption.38}{}}
\newlabel{tab:dirthr@cref}{{[table][12][2147483647]12}{[1][5][]8}}
\newlabel{tab:claimtype}{{13}{8}{\textbf {Claim correctness by type.} The 2,246 atomic claims of the final model's 300 test rationales, judged by GPT-6 Astra with the crop; 24 unverifiable claims are excluded. The weak types are the same ones the judge flagged in the teacher's training text (\cref {tab:errtax})}{table.caption.42}{}}
\newlabel{tab:claimtype@cref}{{[table][13][2147483647]13}{[1][6][]8}}
\newlabel{fig:heads}{{2}{9}{\textbf {The 16 heads of decoder layer 15} at the position where the planner writes the subject cell. Each block is one cell word: the upper row shows the crop and heads 0--7, the lower row the subject mask and heads 8--15. For each word we take the first crop of the evaluation half that received it and has a usable mask; crops were not picked by looking at the maps. The three words whose crop is in portrait format (upper center, center left, center) are left out for space. Heads 1, 6 and 11 (pink) follow the subject mask most closely. The AUC under each head number is the mean over 96 crops}{figure.caption.45}{}}
\newlabel{fig:heads@cref}{{[figure][2][2147483647]2}{[1][7][]9}}
\newlabel{sec:app_limits}{{G.7}{9}{\texorpdfstring {\hskip -1em.~}{}Further limitations}{subsection.G.7}{}}
\newlabel{sec:app_limits@cref}{{[subappendix][7][2147483647,7]G.7}{[1][9][]9}}
\newlabel{fig:heads_auc}{{3}{10}{\textbf {Subject AUC per head.} Left: the 16 heads of decoder layer 15, with the adapter (pink) and without LoRA (gray; the base \vlm on the same input and output); error bars are 95\% bootstrap intervals over 96 crops. Blue dashed line: center prior (0.635); blue dotted line: chance (0.5). Right: all 128 heads of the 8 full-attention layers; values are printed for heads that reach 0.80}{figure.caption.46}{}}
\newlabel{fig:heads_auc@cref}{{[figure][3][2147483647]3}{[1][7][]10}}
\newlabel{tab:generation}{{14}{10}{\textbf {Outpainting backend with the planner fixed.} 100 canvases (44 hand-cropped real photographs, a fixed earlier set of 46 minus the two crops of one statue photograph, which are left out of the image metrics (GPT declined one of them; counted under Refused / blank), plus 56 test crops), same canvases and prompt. This outpainter set is an earlier, separate subset of the manually cropped real-image set of \cref {sec:app_realworld}. All rows are the outpainters' raw outputs, as used throughout the paper; kept-region LPIPS measures how much the outpainter changes the input region; KID compares fills with the real photographs; the seam ratio is a weak proxy for visible seams; fill-vs-GT LPIPS is for reference only, as a plausible fill need not match the reference frame. Human-judged failure is a blind check of 60 raw outputs by the first author, re-weighted to 100 per outpainter. The last two rows add two open masked inpainters run on the same 16\,GB GPU as the rest, also for reference and not ranked: Moebius runs only at its native 512$\times $512 and keeps the input pixels itself; the Qwen-Image ControlNet inpainter runs in 4-bit with the per-image descriptive prompts its model card recommends. Bold = best, underline = second per column}{table.caption.47}{}}
\newlabel{tab:generation@cref}{{[table][14][2147483647]14}{[1][7][]10}}
\newlabel{tab:renderer_human}{{15}{10}{\textbf {Blind human check of the outpainters.} The first author judged 60 raw outputs (30 per seam-ratio stratum, outpainter hidden) for seams and other failures; rates are re-weighted to the 100 canvases of \cref {tab:generation}. The automatic seam ratio ($>$1.5) agrees with the human on 61.7\% of outputs ($\kappa $ 0.23): of the 14 flagged FLUX outputs in the sample, 11 look seamless to a person}{table.caption.48}{}}
\newlabel{tab:renderer_human@cref}{{[table][15][2147483647]15}{[1][7][]10}}
\newlabel{fig:renderer}{{4}{11}{\textbf {Outpainter failures on the same canvases.} (a) the canvas planned by our model (gray = region to fill), filled by (b) GPT Image 2.5, (c) FLUX.1 Fill [dev], (d) SDXL Inpainting 0.1, (e) Moebius and (f) Qwen-Image with the InstantX ControlNet inpainter (*CN = ControlNet), given a per-image descriptive prompt. FLUX invents a sign with gibberish text (top) and leaves the fill blank (bottom); SDXL adds people and text (top) and a title card with a frame (bottom); Moebius, run at its native 512$\times $512, adds a wooden post (top) and meets the input at visible seams; Qwen-Image + CN leaves noise over the whole image and a seam at the input border. GPT completes both scenes without a visible failure. The declined request counted for GPT in \cref {tab:generation} produces no image and is not shown}{figure.caption.49}{}}
\newlabel{fig:renderer@cref}{{[figure][4][2147483647]4}{[1][7][]11}}
\newlabel{tab:metricval}{{16}{11}{\textbf {Can automatic scorers evaluate re-expansion?} Seven pretrained aesthetic or composition scorers on the 300 test crops; every canvas is cut from the real source photograph, no generated pixels. \emph {Ref.\ $>$ crop}: share of crops on which the scorer prefers the complete photograph to its cropped input (95\% bootstrap interval over photos). \emph {Spearman $\rho $}: mean within-image rank correlation between a scorer's score and canvas IoU over the four planners' canvases (\anon {}, \anonnum {}, Claude Opus 5.5 (w/ ICL), constant expansion). \emph {IoU agreement}: share of planner pairs with an IoU gap $\geq 0.05$ on which the scorer prefers the higher-IoU canvas. Brackets: 95\% bootstrap intervals over photos. A canvas that reaches outside the source photograph is clipped before scoring (12\% of the area for \anon {}, 21\% for the constant expansion on average), so the last column repeats $\rho $ against the IoU of the clipped canvas, the geometry the scorer actually saw (clipped-canvas IoU: \anon {} 0.880, \anonnum {} 0.882, Opus 0.818, constant 0.846). SAMP-Net scores 0.74 on the CADB-sourced crops and 0.57 elsewhere; our CADB test crops come from the CADB official test split, which SAMP-Net did not train on}{table.caption.51}{}}
\newlabel{tab:metricval@cref}{{[table][16][2147483647]16}{[1][7][]11}}
\newlabel{sec:app_prompts}{{H}{12}{\texorpdfstring {\hskip -1em.~}{}Prompts}{appendix.H}{}}
\newlabel{sec:app_prompts@cref}{{[appendix][8][2147483647]H}{[1][12][]12}}
\makeatother
